# Supplementary material for: TinyTurbo: Efficient Turbo Decoders on Edge
Source: arXiv:2209.15614 source file (2022-09-30)
Supplement: Supplementary file 1 [file appendix.tex]

% !TEX root = main.tex

\section{Appendix}
\label{sec:appendix}

\subsection{Augmenting MAP decoder}

In Section \ref{sec:results} we saw that \tinyturbo achieves a significant gain over the max-log-MAP decoder. We now evaluate the performance of using \tinyturbo to augment the MAP decoder. We train the \tinyturbo for Turbo$(40,132)$ on the AWGN channel at $-1$ dB, employing the MAP BCJR algorithm. We evaluate the performance of these weights on Turbo$(40,132)$, and Turbo$(200,612)$ codes on the AWGN channel. As shown in in Figs. \ref{fig:bl40_map}, \ref{fig:bl200_map}, we achieve a performance gain by using \tinyturbo to scale the MAP decoder.

\begin{figure}[htbp]
  \centerline{\subfigure[Turbo(40,132)]{  \includegraphics[width=0.25\textwidth]{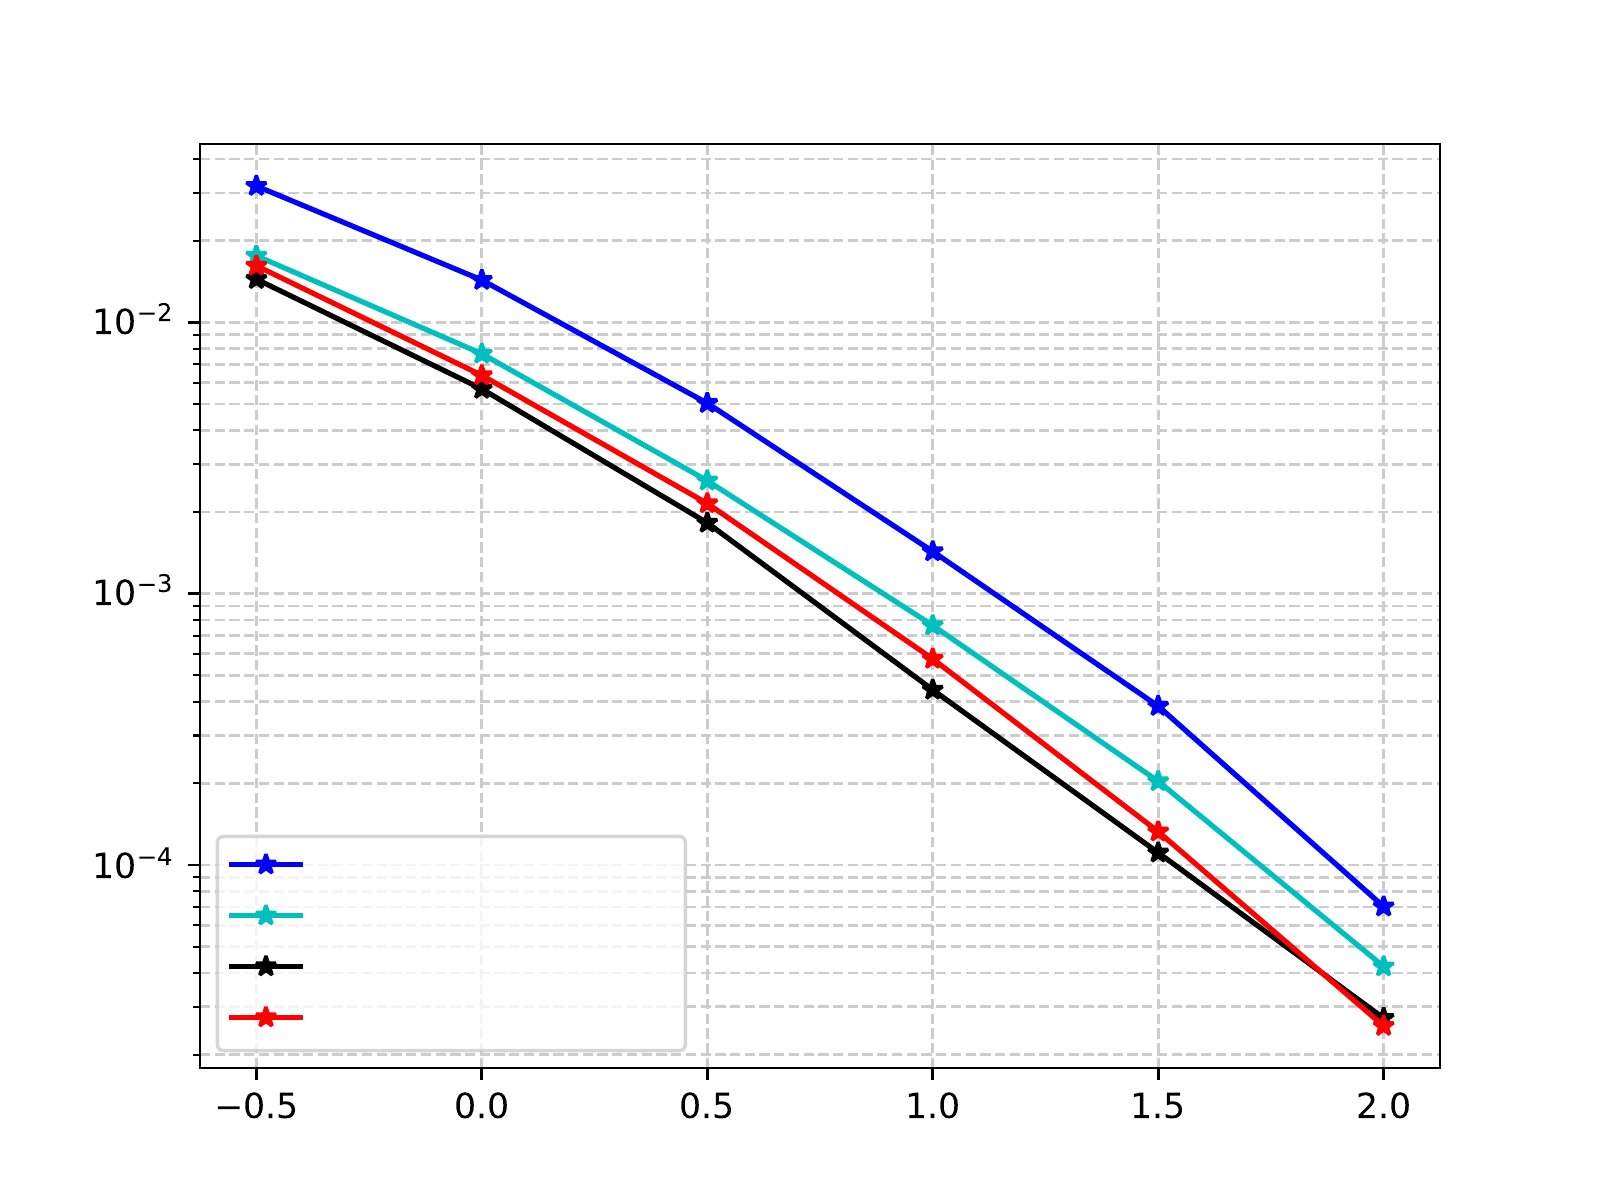}
    \put(-102,26){\fontsize{3}{5}\selectfont max-log-MAP, 3 iters}
    \put(-102,22){\fontsize{3}{5}\selectfont MAP, 3 iters}
    \put(-102,18){\fontsize{3}{5}\selectfont MAP, 6 iters}
    \put(-102,14){\fontsize{3}{5}\selectfont \tinyturbo}
    \put(-100,0){{\fontsize{7}{5}\selectfont Signal-to-noise ratio (SNR)}}
    \put(-127,40){\rotatebox[origin=t]{90}{{\fontsize{5}{5}\selectfont Error rate}}}
    \label{fig:bl40_map}}
    \hfil
    \subfigure[Turbo(200,612) ]{\includegraphics[width=0.25\textwidth]{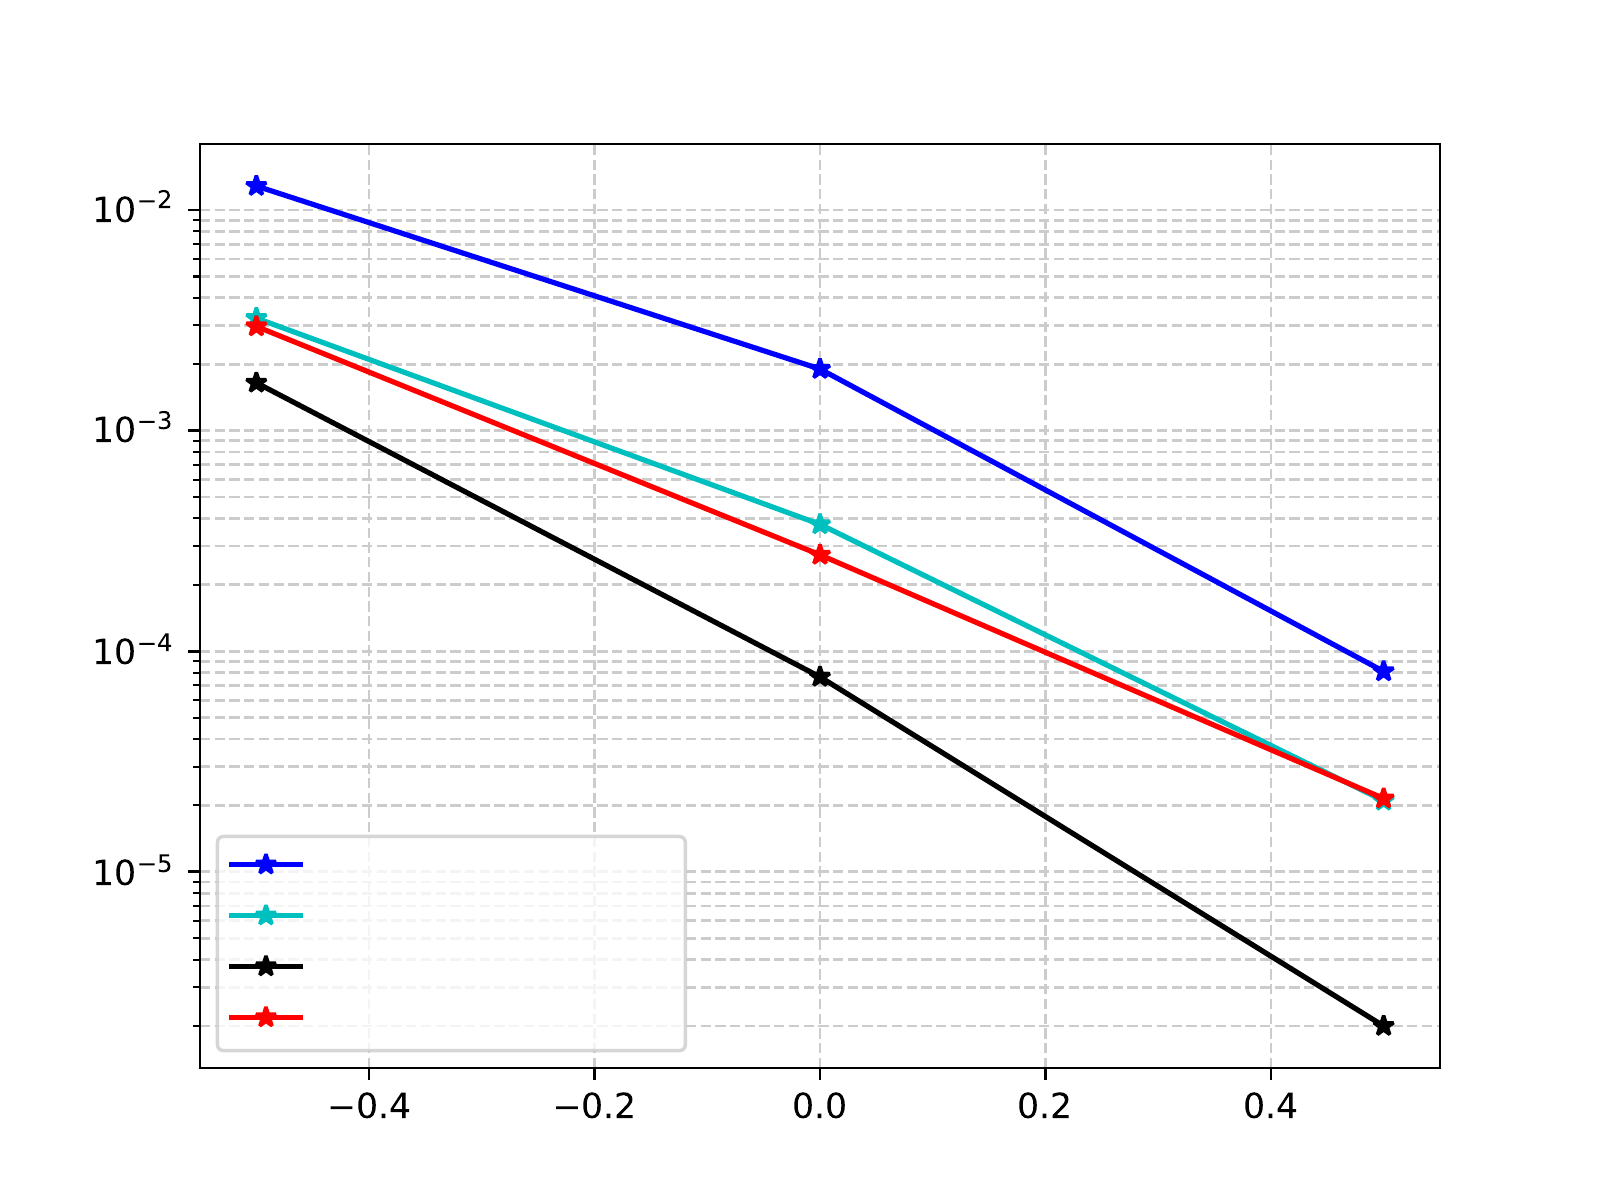}

    \put(-102,26){\fontsize{3}{5}\selectfont max-log-MAP, 3 iters}
    \put(-102,22){\fontsize{3}{5}\selectfont MAP, 3 iters}
    \put(-102,18){\fontsize{3}{5}\selectfont MAP, 6 iters}
    \put(-102,14){\fontsize{3}{5}\selectfont \tinyturbo}
    \put(-100,0){{\fontsize{7}{5}\selectfont Signal-to-noise ratio (SNR)}}
    \put(-127,40){\rotatebox[origin=t]{90}{{\fontsize{5}{5}\selectfont Error rate}}}
    \label{fig:bl200_map}}
    }
    \caption{\tinyturbo trained upon a MAP decoder marginally outperforms the MAP decoding performance with 3 decoding iterations}
\end{figure}

\subsection{Scaling to longer blocklengths}
As demonstrated in Section \ref{sec:block_len_gen}, \tinyturbo trained on a Turbo(40,132) is transferable to turbo codes of block lengths 200. However we observe that for even longer blocklengths, \tinyturbo improves the max-log-MAP performance, but does not approach the MAP performance. As shown in Figure \ref{fig:bl1008}, \tinyturbo employed to decode a turbo code of block length 1008 and rate $1/3$ shows gains over the max-log-MAP decoder; however its performance is sub-optimal compared to the MAP decoder.

\begin{figure}[htbp]
  \centerline{\includegraphics[width=0.25\textwidth]{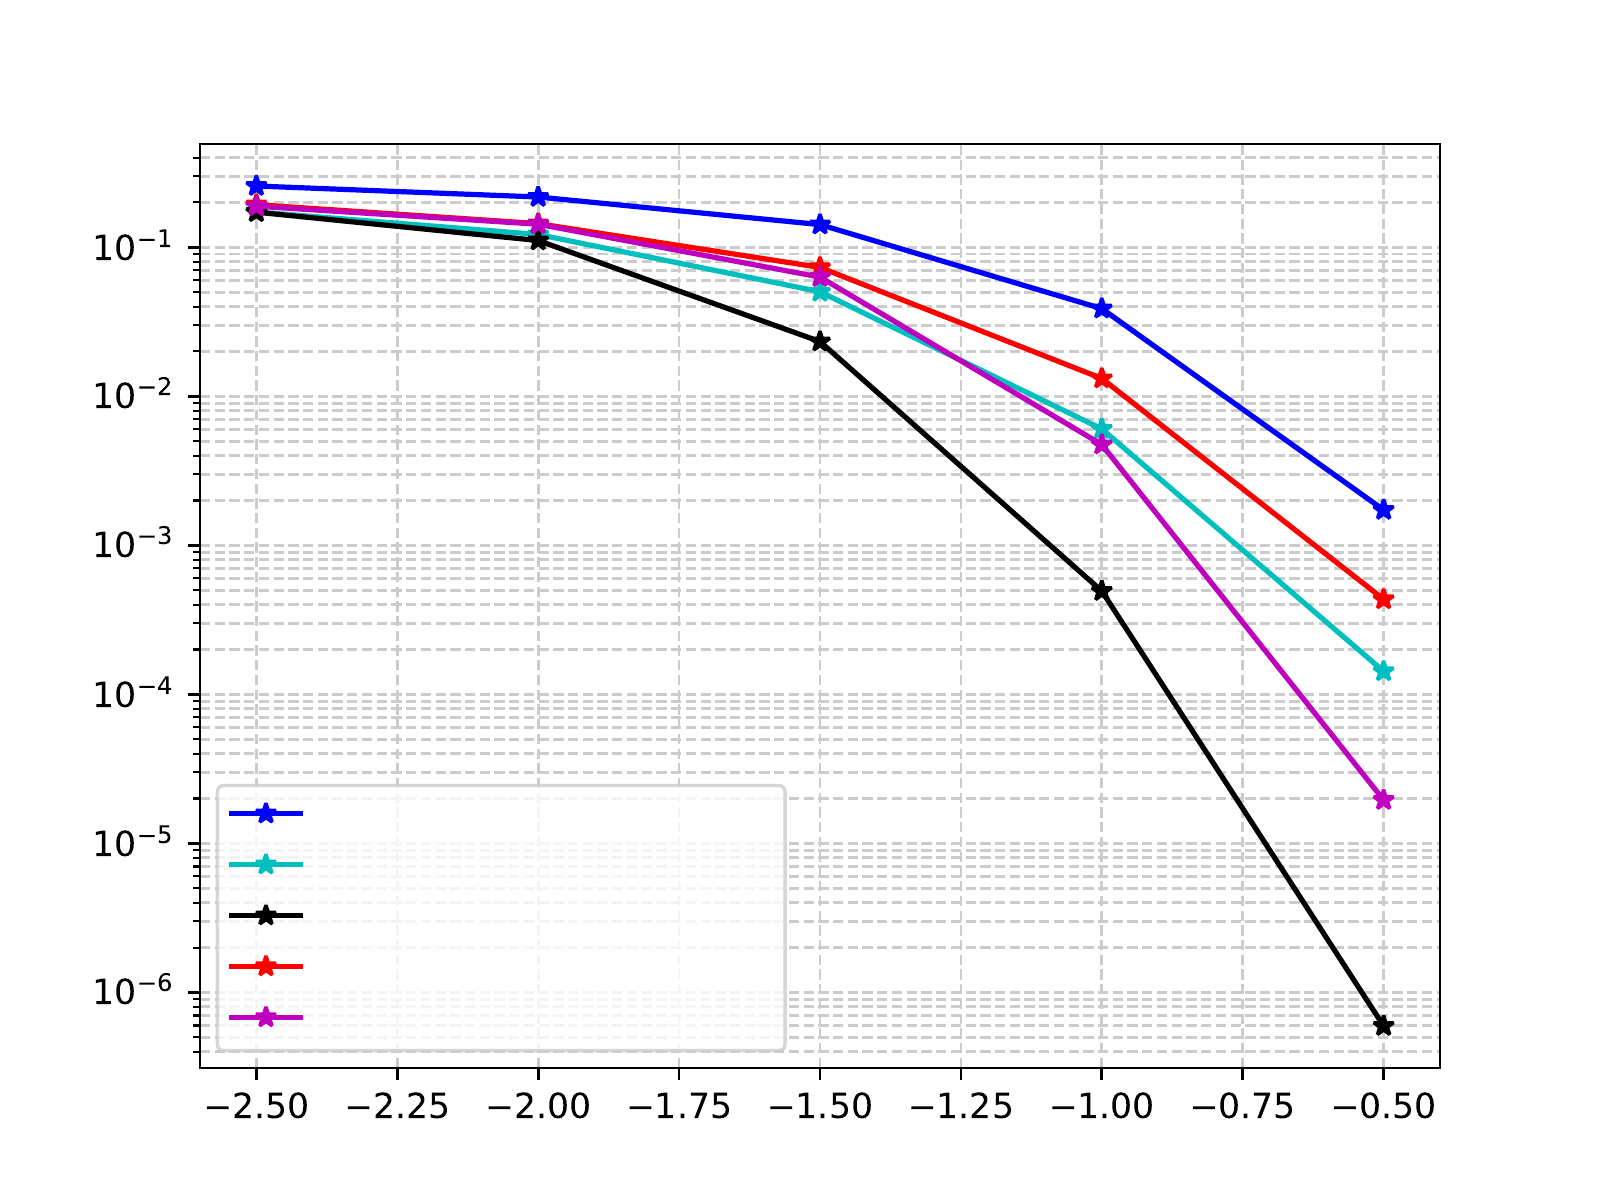}
    \put(-102,30){\fontsize{3}{5}\selectfont max-log-MAP, 3 iters}
    \put(-102,26){\fontsize{3}{5}\selectfont MAP, 3 iters}
    \put(-102,22){\fontsize{3}{5}\selectfont MAP, 6 iters}
    \put(-102,18){\fontsize{3}{5}\selectfont \tinyturbo, 3 iters}
    \put(-102,14){\fontsize{3}{5}\selectfont \tinyturbo, 6 iters}
    \put(-100,0){{\fontsize{7}{5}\selectfont Signal-to-noise ratio (SNR)}}
    \put(-127,40){\rotatebox[origin=t]{90}{{\fontsize{5}{5}\selectfont Error rate}}}}
    \caption{\tinyturbo tested on Turbo(1008, 3036) improves upon max-log-MAP, but is worse compared to MAP}
    \label{fig:bl1008}
\end{figure}

\newpage
